# Supplementary material for: Partnering with Generative AI: Experimental Evaluation of Human-Led and Model-Led Interaction in Human-AI Co-Creation
Source: arXiv:2510.23324 source file (2026-03-09)
Supplement: Supplementary file 1 [file appendix_questionnaire.tex]

% Appendix: Task Description and Questionnaire
% This file can be included with: \input{Analysis/tex tables/appendix_questionnaire}

\section*{Appendix}

\subsection*{Task Description (verbatim)}
\begin{verbatim}
Come up with a creative way to repurpose existing car features—such as cameras, sensors, screens, lights, or speakers—for entirely new uses beyond their original purpose in vehicles.

This idea can be applied inside the vehicle in new ways or outside of the automotive context altogether.

Your goal: Reimagine how this technology could serve new functions, solve problems, or create novel experiences in completely different settings.

Important: Please do not use AI like ChatGPT at this point of the task. We want to see your own creative ideas.
\end{verbatim}

\subsection*{Questionnaire Items and Response Scales}

\subsubsection*{Creative Self-Efficacy}
Scale: 1 = Strongly Disagree, 7 = Strongly Agree
\begin{enumerate}
  \item I was good at coming up with novel ways to repurpose vehicle features.
  \item I had confidence in my ability to solve problems creatively while working on the creativity task.
  \item To ensure you are reading carefully, please select Option 2 for this question. % attention check
  \item I had a knack for further developing the ideas in this exercise.
\end{enumerate}

\subsubsection*{Perceived Technology Agency}
Scale: 1 = Strongly Disagree, 5 = Strongly Agree
\begin{enumerate}
  \item The chatbot goes its own way.
  \item The chatbot does things by itself.
  \item The chatbot takes initiative.
  \item The user of this chatbot does not have to bother about this chatbot a lot.
  \item The chatbot works independently.
\end{enumerate}

\subsubsection*{NASA-TLX (Workload)}
Scale: 0 = very low, 100 = very high (slider)
\begin{enumerate}
  \item How mentally demanding was the task?
  \item How hard did you have to work to accomplish your level of performance?
\end{enumerate}

\subsubsection*{Performance Expectancy}
Scale: 1 = Strongly Disagree, 7 = Strongly Agree
\begin{enumerate}
  \item I find the chatbot useful for creative tasks.
  \item Using the chatbot helps me arrive at creative ideas more quickly.
  \item Using the chatbot increases my productivity when I am working on creative tasks.
\end{enumerate}

\subsubsection*{Effort Expectancy}
Scale: 1 = Strongly Disagree, 7 = Strongly Agree
\begin{enumerate}
  \item Overall, I believe the chatbot is easy to use.
  \item Learning how to use the chatbot for the creativity task is easy for me.
  \item My interactions with the chatbot are clear and understandable.
  \item It is easy for me to become skillful at using the chatbot for creativity tasks.
\end{enumerate}

\subsubsection*{Hedonic Motivation}
Scale: 1 = Strongly Disagree, 7 = Strongly Agree
\begin{enumerate}
  \item I think using the chatbot is fun.
  \item I think using the chatbot is very entertaining.
  \item I think using the chatbot is enjoyable.
\end{enumerate}

\subsubsection*{AI Experience}
Scale: 1 = Never, 2 = Rarely, 3 = Sometimes, 4 = Often, 5 = Daily
\begin{enumerate}
  \item How often do you use AI systems like ChatGPT during the week?
\end{enumerate}

\subsubsection*{Propensity to Trust Technology}
Scale: 1 = Strongly Disagree, 5 = Strongly Agree
\begin{enumerate}
  \item I usually trust AI-powered chatbots until there is a reason not to.
  \item For the most part, I distrust AI-powered chatbots.
  \item In general, I would rely on an AI-powered chatbot to assist me.
  \item This is an attention check question. Please select Strongly Agree (option 5) to show you are paying attention. % attention check
  \item My tendency to trust AI-powered chatbots is high.
  \item It is easy for me to trust AI-powered chatbots to do their job.
  \item I am likely to trust AI-powered chatbots even when I have little knowledge about it.
\end{enumerate}

\subsubsection*{Idea Ownership}
Scale: 1 = Strongly Disagree, 7 = Strongly Agree
\begin{enumerate}
  \item I feel like I am the creator of the idea.
  \item I am the main contributor to the content of the resulting idea.
  \item I have made substantial contributions to the content of the resulting idea.
  \item I am accountable for all aspects of the idea.
  \item I am responsible for at least part of the idea.
\end{enumerate}
